# Supplementary material for: Extending Challenge Sets to Uncover Gender Bias in Machine Translation: Impact of Stereotypical Verbs and Adjectives
Source: arXiv:2107.11584 source file (2021-07-24)
Supplement: Supplementary file 1 [file Appendix__Gender_Bias_in_MT.pdf]

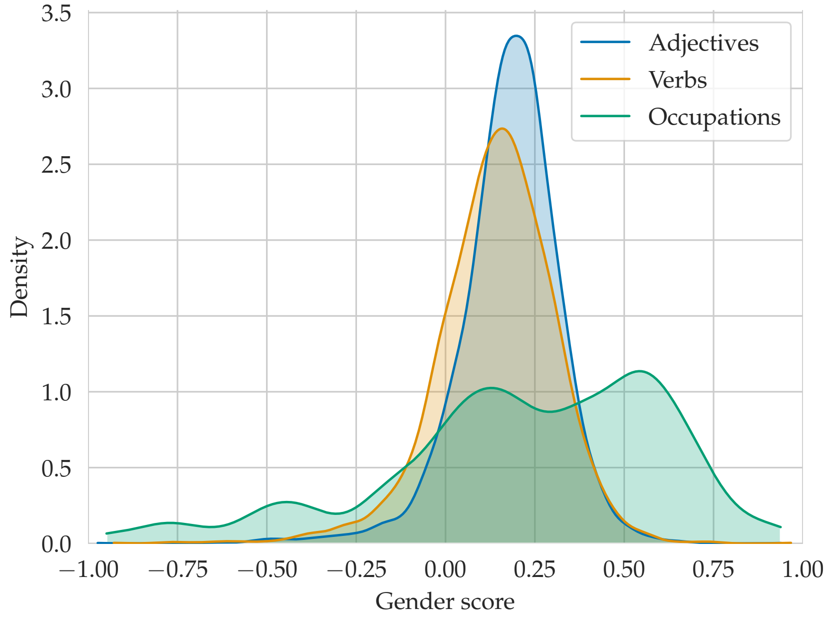


**Fig. 1.** Density plot of the gender score of the three different word-sets: adjectives, verbs, and occupations. The x-axis shows the gender score and the y-axis the density.

# 1 Word Lists

## 1.1 Adjectives

*100 most Feminine:* her, pregnant, mother, matronly, sassy, petite, demure, queenly, motherly, perky, feminine, glamorous, voluptuous, curvy, frumpy, female, brunette, blonde, dress, lovely, coquettish, prenatal, vivacious, dowdy, frilly, prim, maternal, gorgeous, trashy, saucy, beautiful, bubbly, shapely, bewitching, baby, sisterly, sparkly, luscious, statuesque, pink, ravishing, chic, dainty, expectant, enchanting, skimpy, radiant, sensuous, floral, tart, violet, seductive, alluring, clingy, pert, hormonal, bossy, sensual, maiden, satin, reproductive, lacy, cute, adorable, flirtatious, fabulous, foxy, ethereal, brassy, winsome, teeny, scrumptious, filmy, shrieking, delectable, married, giggling, kitchen, teenage, gauzy, sweet, nosy, dressy, yummy, tearful, steamy, unsinkable, hysterical, cooing, shrill, submissive, luminous, vapid, grieving, interracial, fragrant, blooming, prissy, delicious, plump

*100 most Masculine:* his, burly, dapper, grizzled, affable, swaggering, beefy, defensive, cocky, macho, brawny, balding, portly, chief, genial, hulking, pugnacious, genius, jovial, gruff, suave, debonair, doubtful, lanky, coachable,

**Table 1.** The ten most feminine and ten most masculine adjectives that were picked to extend the WinoBias sentences. The *total rank* is the rank the adjectives had in the original list of all 4,762 ranked adjectives. While the *gender scores* seem to differ, the sum of ranks are nearly the same: $sum\_of\_ranks_{feminine} = 284$, $sum\_of\_ranks_{masculine} = 274$.

| feminine adjective | gender score | total rank | masculine adjective | gender score | total rank |
|---|---|---|---|---|---|
| sassy | -0.600 | 5 | grizzled | 0.654 | 4 |
| perky | -0.510 | 10 | affable | 0.648 | 5 |
| brunette | -0.469 | 17 | jovial | 0.557 | 19 |
| blonde | -0.468 | 18 | suave | 0.542 | 21 |
| lovely | -0.452 | 20 | debonair | 0.541 | 22 |
| vivacious | -0.429 | 23 | wiry | 0.517 | 29 |
| saucy | -0.376 | 30 | rascally | 0.515 | 32 |
| bubbly | -0.365 | 32 | arrogant | 0.502 | 42 |
| alluring | -0.267 | 53 | shifty | 0.497 | 45 |
| married | -0.205 | 76 | eminent | 0.480 | 55 |

manly, general, mercenary, wiry, opposing, boastful, rascally, tactical, kingly, mighty, military, rugged, legendary, corrupt, offensive, thundering, arrogant, soldierly, rakish, shifty, master, greatest, game, philosophical, professorial, reputed, signed, scruffy, rank, eminent, managerial, peaceable, lithographic, regimental, pompous, decisive, handsome, theological, latter, prolific, bellicose, incorruptible, unquestioned, mercurial, forged, colossal, topographical, fatherly, muscular, overrated, effeminate, influential, technical, hotheaded, dandy, bellowing, sagacious, irascible, probable, great, blundering, solid, decent, overconfident, brutish, wily, questionable, nationalistic, commanding, cowardly, rotund, shrewd, smarmy, elite, jocular

### 1.2 Verbs

*100 most Feminine:* nurse, dress, crochet, skirt, lace, sew, baby, sass, manicure, accessorize, perfume, bake, embroider, shimmer, fashion, primp, sparkle, gossip, shriek, abort, cake, flower, dance, undress, divorce, escort, model, muse, purse, plump, braid, milk, glitter, pout, giggle, enchant, pamper, marry, beautify, stitch, cruise, intern, knit, bewitch, twirl, blossom, wed, flirt, allure, massage, cackle, sob, spice, miss, brood, slit, conceive, litter, decorate, distress, adore, shower, scream, bleach, love, care, pop, bloom, audition, glaze, weave, shelter, comfort, seduce, nest, kiss, whirl, bustle, cook, blush, pucker, beach, cuddle, scent, broach, swirl, caress, totter, sue, dote, butter, snuggle, clasp, purr, incubate, skin, overeat, carpet, accentuate

*100 most Masculine:* man, engineer, draft, tackle, swagger, captain, team, trade, mastermind, command, corrupt, outlaw, prosper, master, brawl, reckon, marshal, preach, cap, lumber, sanction, guard, build, rank, bankroll, deal, muscle,

**Table 2.** The 21 most feminine and 21 most masculine words that were picked for the verb sentences. The *total rank* is the rank the verbs had in the original list of all 3,210 ranked verbs. While the *gender scores* seem to differ, the sums of ranks are nearly the same: $sum\_of\_ranks_{feminine} = 673$, $sum\_of\_ranks_{masculine} = 675$.

| feminine verb | gender score | total rank | masculine verb | gender score | total rank |
|---|---|---|---|---|---|
| crochet | -0.772 | 3 | draft | 0.733 | 3 |
| sew | -0.646 | 5 | tackle | 0.729 | 4 |
| accessorize | -0.578 | 9 | swagger | 0.677 | 5 |
| bake | -0.516 | 11 | trade | 0.607 | 8 |
| embroider | -0.483 | 12 | brawl | 0.557 | 15 |
| primp | -0.445 | 15 | reckon | 0.549 | 16 |
| gossip | -0.432 | 17 | preach | 0.544 | 18 |
| shriek | -0.411 | 18 | sanction | 0.540 | 21 |
| dance | -0.397 | 22 | build | 0.531 | 23 |
| undress | -0.389 | 23 | boast | 0.496 | 30 |
| milk | -0.360 | 31 | gamble | 0.488 | 36 |
| giggle | -0.351 | 34 | succeed | 0.483 | 38 |
| marry | -0.328 | 37 | regard | 0.483 | 39 |
| knit | -0.309 | 42 | retire | 0.481 | 40 |
| twirl | -0.304 | 44 | chuck | 0.475 | 43 |
| wed | -0.300 | 46 | overthrow | 0.474 | 45 |
| flirt | -0.299 | 47 | rev | 0.472 | 47 |
| allure | -0.298 | 48 | resign | 0.468 | 51 |
| shower | -0.266 | 61 | apprehend | 0.452 | 62 |
| seduce | -0.243 | 73 | appoint | 0.446 | 65 |
| kiss | -0.233 | 75 | fool | 0.445 | 66 |

pitch, sideline, boast, snare, bankrupt, recruit, unify, sack, gamble, prime, succeed, regard, retire, govern, bet, chuck, blunder, overthrow, coach, rev, defeat, excise, huddle, resign, sign, rob, revolt, butcher, respect, mob, amass, warrant, rule, dispossess, apprehend, pipe, score, appoint, fool, reign, prop, nick, fight, sport, doubt, thrash, repute, fumble, humble, slump, plow, position, bribe, degenerate, rival, nickname, dispute, conduct, bat, compromise, kid, roar, quote, cement, surpass, expound, bait, steer, stump, parley, forward, stock, club

### 1.3 Bolukbasi Gender Words

The gender specific words from [1]. Sorted and split into a feminine list and a masculine list:

*Female:* her, she, women, woman, wife, mother, daughter, girls, girl, spokeswoman, female, sister, herself, actress, mom, girlfriend, daughters, lady, sisters, mothers, grandmother, ladies, queen, ma, wives, widow, bride, females, aunt, lesbian, chairwoman, moms, maiden, granddaughter, niece, hers, filly,

princess, lesbians, actresses, maid, mare, fiancee, waitress, maternal, heroine, nieces, girlfriends, mistress, womb, grandma, maternity, estrogen, widows, diva, nuns, nun, brides, housewife, menopause, motherhood, stepmother, hostess, fillies, congresswoman, witch, sorority, businesswoman, gal, schoolgirl, goddess, stepdaughter, uterus, mama, hens, hen, mommy, grandmothers, feminism, heiress, queens, witches, aunts, granddaughters, convent, vagina, maids, gals, housewives, obstetrics, councilwoman, matriarch, dowry, deer

*Male:* he, his, him, man, men, spokesman, himself, son, father, guy, boy, boys, brother, male, brothers, dad, dads, sons, king, businessman, grandfather, uncle, congressman, grandson, bull, businessmen, nephew, fathers, lads, lion, gentleman, fraternity, bachelor, bulls, prince, colt, salesman, dude, beard, councilman, gentlemen, stepfather, monks, lad, testosterone, nephews, daddy, kings, sir, stud, lions, gelding, czar, countrymen, penis, bloke, spokesmen, monastery, brethren, schoolboy, brotherhood, stepson, uncles, monk, viagra, macho, statesman, fathered, blokes, dudes, strongman, grandsons, studs, godfather, boyhood, baritone, grandpa, countryman, stallion, fella, chap, widower, salesmen, beau, beards, handyman, horsemen, fatherhood, princes, colts, fraternities, pa, fellas, councilmen, barbershop, fraternal, husband, boyfriend, males, husbands, sperm, fiance, suitors, prostate, paternity, suitor, hubby, boyfriends, semen

## 2 Verb Sentences

All 42 verb-sentences with placeholders for occupational nouns:

| Gender | Verb | Sentence |
|---|---|---|
| F | crochet | The X crochets potholders. |
| F | sew | The X sews a new T-shirt. |
| F | accessorize | The X accessorizes the workspace. |
| F | bake | The X bakes a cake. |
| F | embroider | The X embroiders a shirt. |
| F | primp | The X primps up the room for a showing. |
| F | gossip | The X gossips with colleagues. |
| F | shriek | The X shrieks when seeing the spider. |
| F | dance | The X dances in the club. |
| F | undress | The X undresses for examination. |
| F | milk | The X milks a cow on vacation. |
| F | giggle | The X giggles over a joke. |
| F | marry | The X marries on a Saturday. |
| F | knit | The X knits a pullover. |
| F | twirl | The X twirls a friend round the dance floor. |
| F | wed | The X weds on a sunday. |
| F | flirt | The X flirts with a coworker. |
| F | allure | The X allures a coworker. |
| F | shower | The X showers after work. |
| F | seduce | The X seduces a colleague. |
| F | kiss | The X kisses a colleague. |
| M | draft | The X drafts a corona-handout. |
| M | tackle | The X tackles all problems. |
| M | swagger | The X swaggers about the new bike. |
| M | trade | The X trades the old phone up. |
| M | brawl | The X brawls with a coworker. |
| M | reckon | The X reckons up the total sum. |
| M | preach | The X preaches caution. |
| M | sanction | The X sanctions the deal. |
| M | build | The X builds confidence at work. |
| M | boast | The X boasts about the new car. |
| M | gamble | The X gambles away 20 dollar. |
| M | succeed | The X succeeds in the exam. |
| M | regard | The X regards a colleague with favour. |
| M | retire | The X retires after 40 years. |
| M | chuck | The X chucks away old shoes. |
| M | overthrow | The X overthrows a colleague in a fight. |
| M | rev | The X revs the car engine. |
| M | resign | The X resigns because of bad working conditions. |
| M | apprehend | The X apprehends the explanation. |
| M | appoint | The X appoints a date for the meeting. |
| M | fool | The X fools the boss. |

## 3 Overview of Complete Process

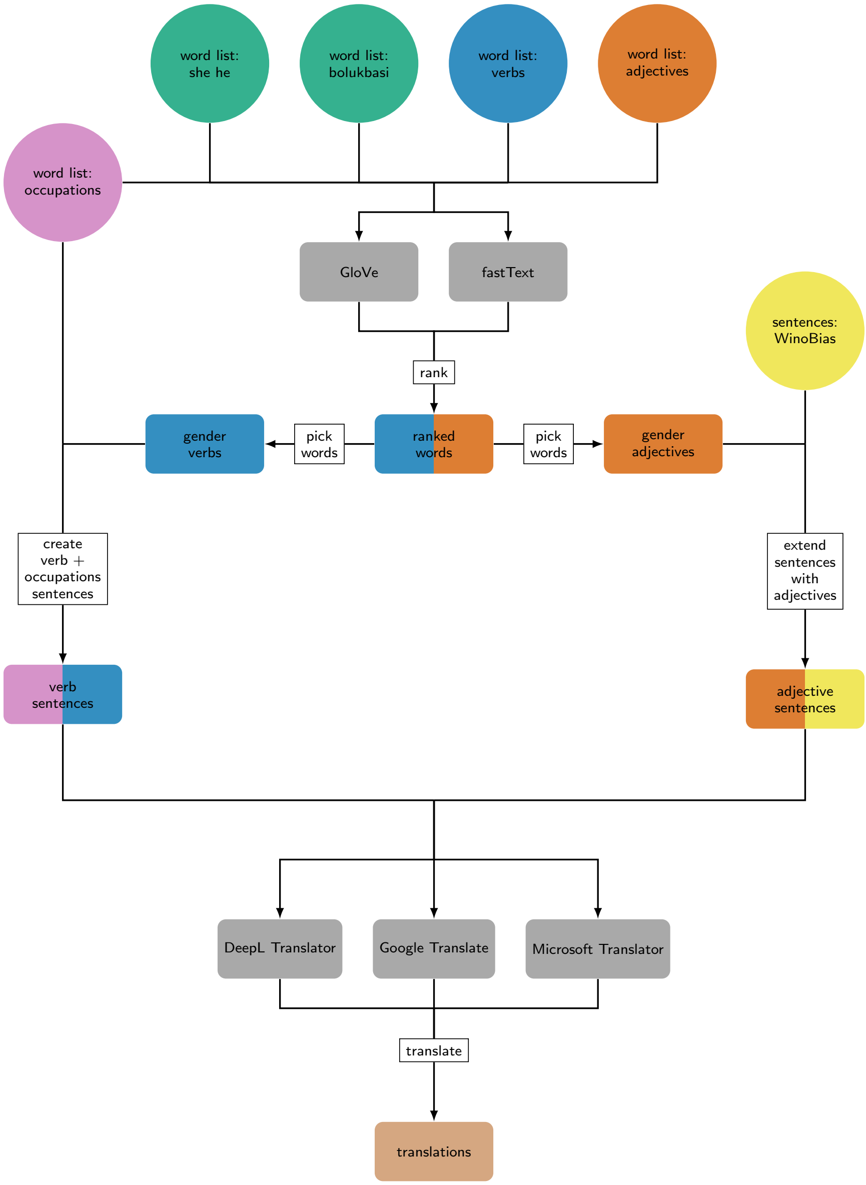


**Fig. 2.** Illustration of all data and methods used to create, translate, evaluate, and extend the WiBeMT challenge set. Circles resemble input data, grey rectangles resemble word embeddings and MT systems, colored rectangles resemble processed data, and white rectangles resemble processes.

## References

1. Bolukbasi, T., Chang, K.W., Zou, J., Saligrama, V., Kalai, A.: Man is to computer programmer as woman is to homemaker? Debiasing word embeddings. Advances in Neural Information Processing Systems pp. 4356–4364 (2016)
